# Supplementary material for: Dr. Strategy: Model-Based Generalist Agents with Strategic Dreaming
Source: arXiv:2402.18866 source file (2024-06-04)
Supplement: Supplementary file 1 [file A_QuantitativeResults.tex]

\section{Quantitative results}

\begin{center}
    \begin{table}[h]
        \centering
        \begin{tabular}{ lp{1.5cm}p{1.5cm}p{1.5cm}p{1.9cm}p{1.9cm}p{1.9cm}l  }
        \toprule
        \textbf{Method} & \centering \textbf{9-Room} & \centering \textbf{Spiral 9-Room} & \centering \textbf{25-Room} & \centering \textbf{Maze-7x7}& \centering \textbf{Maze-15x15} & \centering \textbf{RoboKitchen} &\\
        \midrule
         \vspace{0.5em}
         LEXA & \centering 19.75\% & \centering 21.19\% & \centering 9.62\% & \centering 51.11\% & \centering 41.20\% & \centering \textbf{24.30\%} &\\
         \vspace{0.5em}
         LEXA-expl & \centering 16.04\% & \centering 20.16\% & \centering 0.14\% & \centering 43.70\% & \centering 18.05\% & \centering 20.07\% &\\
         \vspace{0.5em}
         GC-Director & \centering 28.08\% & \centering 30.45\% & \centering 27.11\% & \centering 40.55\% & \centering 21.87\% & \centering 1.45\% &\\
         \toprule
         \centering \textbf{Dr. Strategy(Ours)} & \centering \textbf{94.03\%} & \centering \textbf{96.50\%} & \centering \textbf{67.11\%} & \centering \textbf{86.66\%}& \centering \textbf{44.44\%} & \centering 19.44\% &\\
        \bottomrule
        \end{tabular}
    \caption{Full table of the quantative results}
    \end{table}
\end{center}
